# Supplementary material for: Using LLMs to discover emerging coded antisemitic hate-speech in extremist social media
Source: arXiv:2401.10841 source file (2024-01-23)
Supplement: Supplementary file 1 [file Appendix.tex]

\subsection{Appendix}
\begin{algorithm}[h]
	\caption{Extracting Embedding for standard method}
	\begin{algorithmic}[1]
            \State Trending\_terms \gets $[$t_1, t_2,\dots, t_n$]$\Comment{Trending bigrams/trigrams of length n}
            \State Glossary \gets $[$g_1,g_2,\dots,g_{m}$]$\Comment{Total Seed words used of length m}
            \State Uncleaned\_text \gets $[$post_1,post_2,\dots, post_U$]$\Comment{Totals posts of length U}

            \State Initialize $X_t$ to store trending terms and thier list of context sentences embeddings.
             \State Initialize $X_g$ to store glossary terms and their list of context sentences embeddings.

            %\State Store the terms of the vocabulary in a list ${\bf t}$ \Comment{Length(t) $=$ $V$}
            
		\For {each \textit{term} in ${\bf Trending\_terms}$}
 % \State Initialize $t_h$ \Comment{To store highest TF-IDF score across all $d$ }
            \For{each \textit{post} in ${\bf Uncleaned\_text}$}
              \State {lemmatized\_text \gets Lemmatize(\textit{post})}\Comment{we lemmatize the post as the trending terms are in its base form}
            \If{\textit{term} in ${\bf \textit{lemmatized\_text}}$}
            \State {Extract surrounding words for the \textit{term} with given range and store it as a sentence in p\_t}
            \State {$X_t[term]$ \gets Bert\_Embeddings\ (p\_t)} \Comment{Add the Fine-tuned Bert embeddings of the sentence to the term list.}
            \EndIf
            
            \EndFor

            \EndFor

            \For {each \textit{term} in ${\bf Glossary}$}
 % \State Initialize $t_h$ \Comment{To store highest TF-IDF score across all $d$ }
            \For{each \textit{post} in ${\bf Uncleaned\_text}$}
            \If{\textit{term} in ${\bf \textit{post}}$}
            \State {Extract surrounding words for the \textit{term} with given range and store it as a sentence in p\_t}
            \State {$X_g[term]$ \gets Bert\_Embeddings\ (p\_t)} \Comment{Add the Fine-tuned Bert embeddings of the sentence to the term list.}
            \EndIf
            
            \EndFor

            \EndFor
            \State {Initialize $E_t$ to store trending terms and their associated single embedding. }
            \State Initialize $E_g$ to store glossary terms and their associated single embeddings.
            \For{ each term in $X_t$}
            \State {$E\_t$ \gets Average($X_t[term]$,column=True)}\Comment{Average all the embeddings in the list for the Important terms along the y-axis.}
            \EndFor
            \For{ each term in $X_g$}
            \State $E\_g$ \gets Average($X_g[term]$,column=True)\Comment{Average all the embeddings in the list for the Glossary terms along the y-axis.}
            \EndFor
        \end{algorithmic}
\end{algorithm}

\begin{algorithm}[h]
	\caption{Embedding extraction for advanced method}
	\begin{algorithmic}[1]
            \State Trending\_terms \gets $[$t_1, t_2,\dots, t_n$]$\Comment{Trending bigrams/trigrams of length n}
            \State Glossary \gets $[$g_1,g_2,\dots,g_{m}$]$\Comment{Total Seed words used of length m}
            \State Uncleaned\_text \gets $[$post_1,post_2,\dots,
            post_U$]$\Comment{Total posts of length U}

            \State Initialize $X_t$ to store trending terms and thier list of context embeddings.
            \State Initialize $X_g$ to store glossary terms and their list of context embeddings.

            %\State Store the terms of the vocabulary in a list ${\bf t}$ \Comment{Length(t) $=$ $V$}

            \For{each \textit{post} in ${\bf Uncleaned\_text}$}
            \State {lemmatized\_text \gets Lemmatize(\textit{post})}\Comment{we lemmatize the post as the trending terms are in its base form}
            \State { Text\_Embedding \gets Bert\_Embedding(lemmatized\_text)}\Comment{Run the Bert model on complete lemmatized text}
            
		\For {each \textit{term} in ${\bf Trending\_terms}$}
 % \State Initialize $t_h$ \Comment{To store highest TF-IDF score across all $d$ }
            
            \If{\textit{term} in ${\bf lemmatized\_text}$}
            \State {Extract surrounding words for the \textit{term} with given \texttt{range} and store it in p\_t}
            \State {$X_t[term]$ \gets Average(Text\_Embedding(p\_t)[last layer],column=True)} \Comment{Average the last hidden layer of these words across the columns of length 768.}
            \EndIf
          
            \EndFor

            \EndFor
            \For{each \textit{post} in ${\bf Uncleaned\_text}$}
            \State { Text\_Embedding \gets Bert\_Embedding(\textit{post})}\Comment{}
            \For {each \textit{term} in ${\bf Glossary}$}
 % \State Initialize $t_h$ \Comment{To store highest TF-IDF score across all $d$ }
            
            \If{\textit{term} in ${\bf \textit{post}}$}
            \State {Extract surrounding words for the \textit{term} with given range and store it in p\_t}
            \State {$X_g[term]$ \gets Average(Text\_Embedding(p\_t),column=True)} \Comment{Average the last hidden layer of these words across the columns of length 768.}
            \EndIf
            
            \EndFor

            \EndFor
            \State {Initialize $E_t$ to store trending terms and their associated single embedding. }
            \State Initialize $E_g$ to store glossary terms and their associated single embeddings.
            \For{ each term in $X_t$}
            \State {$E\_t$ \gets Average($X_t[term]$,column=True)}\Comment{Average all the embeddings in the list for the Important terms along the y-axis.}
            \EndFor
            \For{ each term in $X_g$}
            \State $E\_g$ \gets Average($X_g[term]$,column=True)\Comment{Average all the embeddings in the list for the Glossary terms along the y-axis.}
            \EndFor
        \end{algorithmic}
\end{algorithm}

\begin{algorithm}[h]
	\caption{Comparing Semantic Similarity}
	\begin{algorithmic}[1]
            \State Embeddings\_tt \gets \{$t\_1:et\_1$,$t\_2:et\_2$\dots $t\_n:et\_n$\}\Comment{Trending terms after phase 1}
            \State Embeddings\_gt \gets \{$g\_1:eg\_1$,$g\_2:eg\_2$\dots$g\_14:eg\_14$\}\Comment{Total Seed words used of context similarity}
            \State Initialize TT\_PL to store trending terms and their predicted antisemitic label.
            \State Initialize $S_i$ to store single semantic score for each trending term.
		\For {each \textit{tt} in ${\bf Embeddings\_tt}$}
            \For{each \textit{gt} in ${\bf Embeddings\_gt}$}
            \State {Compute the semantic similarity between trending term(tt) with all glossary terms(gt) and store all the scores in tt\_scores}
            \EndFor
            \State {$score$ \gets Average(${tt\_scores}$)} \Comment{Average all the semantic scores between trending term and seed terms and assign a single score to the term}
            \State {$S_i$[tt] \gets score }
        \EndFor

            \State {\gamma \gets Median($S_i$)}
            \For {each \textit{tt} in ${\bf S_i}$}
            \If{$S_i[tt]$ $>$ \gamma}\Comment{check if semantic score for the term in greater than threshold}
            \State {$TT\_PL[tt]$ \gets 1 }\Comment{1 if the score greater than \gamma}
            \Else
            \State {$TT\_PL[tt]$ \gets 0 }\Comment{0 if the score is less than \gamma}
            \EndIf
            \EndFor
        \end{algorithmic}
\end{algorithm}
